# Supplementary material for: Dynamics of particle-laden turbulent Couette flow. Part1: Turbulence modulation by inertial particles
Source: arXiv:2204.00217 source file (2022-04-01)
Supplement: Supplementary file 1 [file appendix.tex]

\chapter{Appendix}
\section{Variation of Inter-particle Collision Frequency in One-way Coupled Turbulent Shear Flow }
\label{app_coll_freq}
	Collision frequency profile is studied for the various DNS runs of chapter \ref{chapt1}. The variation of inter-particle collision frequency is tabulated for various simulation runs as mentioned in the legend of the figure \ref{fig:coll_freq}.
	\begin{figure}[h]
	    \centering
	    \includegraphics[width=0.75\linewidth]{chapt1/Coll_freq.eps}
	    \caption{Variation of Inter-particle Collision Frequency in $U/\delta$ Units as a Function of $y/\delta$; The Different Cases are Shown in Legends }
	    \label{fig:coll_freq}
	\end{figure}
	\clearpage
%------------------------------------------------------
\clearpage	
\section{Derivation of Random Torques Generation}
\label{Derivation of Random Torque Generation}
The formulation of the Random torques is initiated through three independent normal random deviates $\zeta_1$, $\zeta_2$ , $\zeta_3$  of zero mean and unit variance. 
In accordance with equation(\ref{eq2.30}) and replacing $\delta(t-t')=\frac{1}{\Delta t}$ we can write

\begin{eqnarray}
	\label{eq5.33}
	\langle T_x(t)T_x(t)\rangle=\frac{2D_{\Omega{xx}}}{\Delta t}\\
	\label{eq5.34}
	\langle T_y(t)T_y(t)\rangle=\frac{2D_{\Omega{yy}}}{\Delta t}\\
	\label{eq5.35}
	\langle T_z(t)T_z(t)\rangle=\frac{2D_{\Omega{zz}}}{\Delta t}\\
	\label{eq5.36}
	\langle T_x(t)T_y(t)\rangle=\frac{2D_{\Omega{xy}}}{\Delta t}\\
	\label{eq5.37}
	\langle T_x(t)T_z(t)\rangle=\frac{2D_{\Omega{xz}}}{\Delta t}\\
	\label{eq5.38}
	\langle T_y(t)T_z(t)\rangle=\frac{2D_{\Omega{yz}}}{\Delta t}
\end{eqnarray}
In accordance with equation (\ref{eq5.33}) let the fluctuating torque along x be written as:
\begin{equation}
	\label{eq5.39}
	T_x=\frac{\sqrt{2D_{\Omega{xx}}}}{\sqrt{\Delta t}}\zeta_1
\end{equation} 
Now let us consider the functional form of the fluctuating torque along y,such that $T_y$ remains correlated with itself and $T_x$ and the functional form is given as:

\begin{equation}
	\label{eq5.40}
	T_y=\frac{\sqrt{2D_{\Omega{yy}}}}{\sqrt{\Delta t}}[b\zeta_1+c\zeta_2]
\end{equation}
where $a$ and $b$ are two constants

Now multiplying equation (\ref{eq5.39}) and (\ref{eq5.40}) and taking the second moment we get:
\begin{equation}
	\label{eq5.41}
	\langle T_x T_y\rangle=\frac{2}{\Delta t}b\sqrt{D_{\Omega{xx}}D_{\Omega{yy}}}
\end{equation} 
Now, comparing equation (\ref{eq5.41}) with equation (\ref{eq5.36}) we get the value of constant $b$ as:
\begin{equation}
	\label{eq5.42}
	b=\frac{D_{\Omega{xy}}}{\sqrt{D_{\Omega{xx}}D_{\Omega{yy}}}}
\end{equation} 

Simillarly,Now multiplying equation (\ref{eq5.40}) and (\ref{eq5.40}) and taking the second moment we get:
\begin{equation}
	\label{eq5.43}
	\langle T_y T_y\rangle=\frac{2D_{\Omega{yy}}}{\Delta t}[b^2+c^2]
\end{equation}

Now, comparing equation (\ref{eq5.43}) with equation (\ref{eq5.34}) we get the value of constant $b$ as:
\begin{equation}
	\label{eq5.44}
	c=\sqrt{1-b^2}=\sqrt{1-\frac{{D^2}_{\Omega{xy}}}{D_{\Omega{xx}}D_{\Omega{yy}}}}
\end{equation}

So the fluctuating torque along y direction is given by:
\begin{equation}
	\label{eq5.45}
	T_y=\frac{\sqrt{2D_{\Omega{yy}}}}{\sqrt{\Delta t}}\Bigg[\frac{D_{\Omega{xy}}}{\sqrt{D_{\Omega{xx}}D_{\Omega{yy}}}}\zeta_1+ \sqrt{1-\frac{D_{\Omega{xy}}^2}{D_{\Omega{xx}}D_{\Omega{yy}}}}\zeta_2\Bigg]
\end{equation}\\

In order to write the functional form of $T_z$ we have to consider the fact that it is not only correlated with itself but also with $T_x$, and $T_y$. In this way we could capture all the possible second moments given from equation (\ref{eq5.33}) to equation (\ref{eq5.38}).
The functional form of $T_z$ could be written as:

\begin{equation}
	\label{eq5.46}
	T_z=\frac{\sqrt{2D_{\Omega{zz}}}}{\sqrt{\Delta t}}[a_1\zeta_1+a_2\zeta_2+a_3\zeta_3]
\end{equation}
where $a_1$,$a_2$ and $a_3$ are constants to be evaluated.

Now multiplying equation (\ref{eq5.46}) and (\ref{eq5.39}) and taking the second moment we get:
\begin{equation}
	\label{eq5.47}
	\langle T_x T_z\rangle=\frac{2}{\Delta t}a_1\sqrt{D_{\Omega{xx}}D_{\Omega{zz}}}
\end{equation} 

Comparing equation (\ref{eq5.47}) with equation (\ref{eq5.37}) we get the value of constant $a_1$ as:
\begin{equation}
	\label{eq5.48}
	a_1=\frac{D_{\Omega{xz}}}{\sqrt{D_{\Omega{xx}}D_{\Omega{zz}}}}
\end{equation}

In order evaluate the constant $a_2$ we consider the cross-covariance of $T_y$ and $T_z$.
Multiplying equation (\ref{eq5.46}) and (\ref{eq5.45}) and taking the second moment we get:

\begin{equation}
	\label{eq5.49}
	\langle T_y T_z\rangle=\frac{2}{\Delta t}\sqrt{D_{\Omega{yy}}D_{\Omega{zz}}}[a_1\frac{D_{\Omega{xy}}}{\sqrt{D_{\Omega{xx}}D_{\Omega{yy}}}}+a_2\sqrt{1-\frac{D_{\Omega{xy}}^2}{D_{\Omega{xx}}D_{\Omega{yy}}}}]
\end{equation}

Comparing equation (\ref{eq5.49}) with equation (\ref{eq5.38}) we get the value of constant $a_2$ as:

\begin{equation}
	\label{eq5.50}
	a_2=\frac{\frac{D_{\Omega{yz}}}{\sqrt{D_{\Omega{yy}}D_{\Omega{zz}}}}-a_1\frac{D_{\Omega{xy}}}{\sqrt{D_{\Omega{xx}}D_{\Omega{yy}}}}}{\sqrt{1-\frac{D_{\Omega{xy}}^2}{D_{\Omega{xx}}D_{\Omega{yy}}}}}
\end{equation} 

Equation(\ref{eq5.50}) can be alternatively written as:

\begin{equation}
	\label{eq5.51}
	a_2=\frac{\frac{D_{\Omega{yz}}}{\sqrt{D_{\Omega{yy}}D_{\Omega{zz}}}}-\frac{D_{\Omega{xz}}}{\sqrt{D_{\Omega{xx}}D_{\Omega{zz}}}}\frac{D_{\Omega{xy}}}{\sqrt{D_{\Omega{xx}}D_{\Omega{yy}}}}}{\sqrt{1-\frac{D_{\Omega{xy}}^2}{D_{\Omega{xx}}D_{\Omega{yy}}}}}
\end{equation}

Simillarly,Now multiplying equation (\ref{eq5.46}) and (\ref{eq5.46}) and taking the second moment we get:
\begin{equation}
	\label{eq5.52}
	\langle T_z T_z\rangle=\frac{2D_{\Omega{zz}}}{\Delta t}[a_1^2+a_2^2+a_3^2]
\end{equation}

Comparing equation (\ref{eq5.52}) with equation (\ref{eq5.35}) we get the value of constant $a_2$ as:
\begin{equation}
	\label{eq5.53}
	a_3=\sqrt{1-a_1^2-a_2^2}=\sqrt{1-\frac{{D^2}_{\Omega{xz}}}{D_{\Omega{xx}}D_{\Omega{zz}}}-\frac{[\frac{D_{\Omega{yz}}}{\sqrt{D_{\Omega{yy}}D_{\Omega{zz}}}}-\frac{D_{\Omega{xz}}}{\sqrt{D_{\Omega{xx}}D_{\Omega{zz}}}}\frac{D_{\Omega{xy}}}{\sqrt{D_{\Omega{xx}}D_{\Omega{yy}}}}]^2}{[1-\frac{D_{\Omega{xy}}^2}{D_{\Omega{xx}}D_{\Omega{yy}}}]}}
\end{equation}

Equation (\ref{eq5.46}), equation (\ref{eq5.48}), equation (\ref{eq5.51}) and equation (\ref{eq5.53}) together generates the expression of fluctuating torque along z direction , $T_z$.

\begin{eqnarray} 
	\label{eq5.54}
	T_z & = & \frac{\sqrt{2D_{\Omega{zz}}}}{\sqrt{\Delta t}}\left[\frac{D_{\Omega{xz}}}{\sqrt{D_{\Omega{xx}}D_{\Omega{zz}}}}\zeta_1+{\frac{\frac{D_{\Omega{yz}}}{\sqrt{D_{\Omega{yy}}D_{\Omega{zz}}}}-\frac{D_{\Omega{xz}}}{\sqrt{D_{\Omega{xx}}D_{\Omega{zz}}}}\frac{D_{\Omega{xy}}}{\sqrt{D_{\Omega{xx}}D_{\Omega{yy}}}}}{\sqrt{1-\frac{D_{\Omega{xy}}^2}{D_{\Omega{xx}}D_{\Omega{yy}}}}}}\zeta_2+ \right. \nonumber \\
	&& \mbox{}\left.{\sqrt{1-\frac{D_{\Omega{xz}}^2}{D_{\Omega{xx}}D_{\Omega{zz}}}-\frac{\left[\frac{D_{\Omega{yz}}}{\sqrt{D_{\Omega{yy}}D_{\Omega{zz}}}}-\frac{D_{\Omega{xz}}}{\sqrt{D_{\Omega{xx}}D_{\Omega{zz}}}}\frac{D_{\Omega{xy}}}{\sqrt{D_{\Omega{xx}}D_{\Omega{yy}}}}\right]^2}{\left[1-\frac{D_{\Omega{xy}}^2}{D_{\Omega{xx}}D_{\Omega{yy}}} \right]}}}\zeta_3 \right]                                                               
\end{eqnarray}
%------------------------------------------------------
\clearpage
\section{Particle Phase Statistics in two-way Coupled Turbulent Shear Flow}
\label{sec:Particle Phase Statistics}
Particle phase statistics for two different cases with different collisional conditions: slightly inelastic inter-particle and wall-particle collisions with ($e=0.9$) and inter-particle collisions being switched-off, are presented here in addition to the perfectly elastic inter-particle and wall-particle collisions presented in chapter \ref{chapt4}, section \ref{sec:Particle Phase Statistics ideal}. 
\subsection{Perfectly Elastic Inter-particle and Wall-particle Collisions}

\subsection{Inelastic Inter-particle and Wall-particle Collisions}
\label{sec:Particle Phase Statistics inelastic}
\begin{figure}[!h]
			\includegraphics[width=1.0\textwidth,  height=9cm]{app/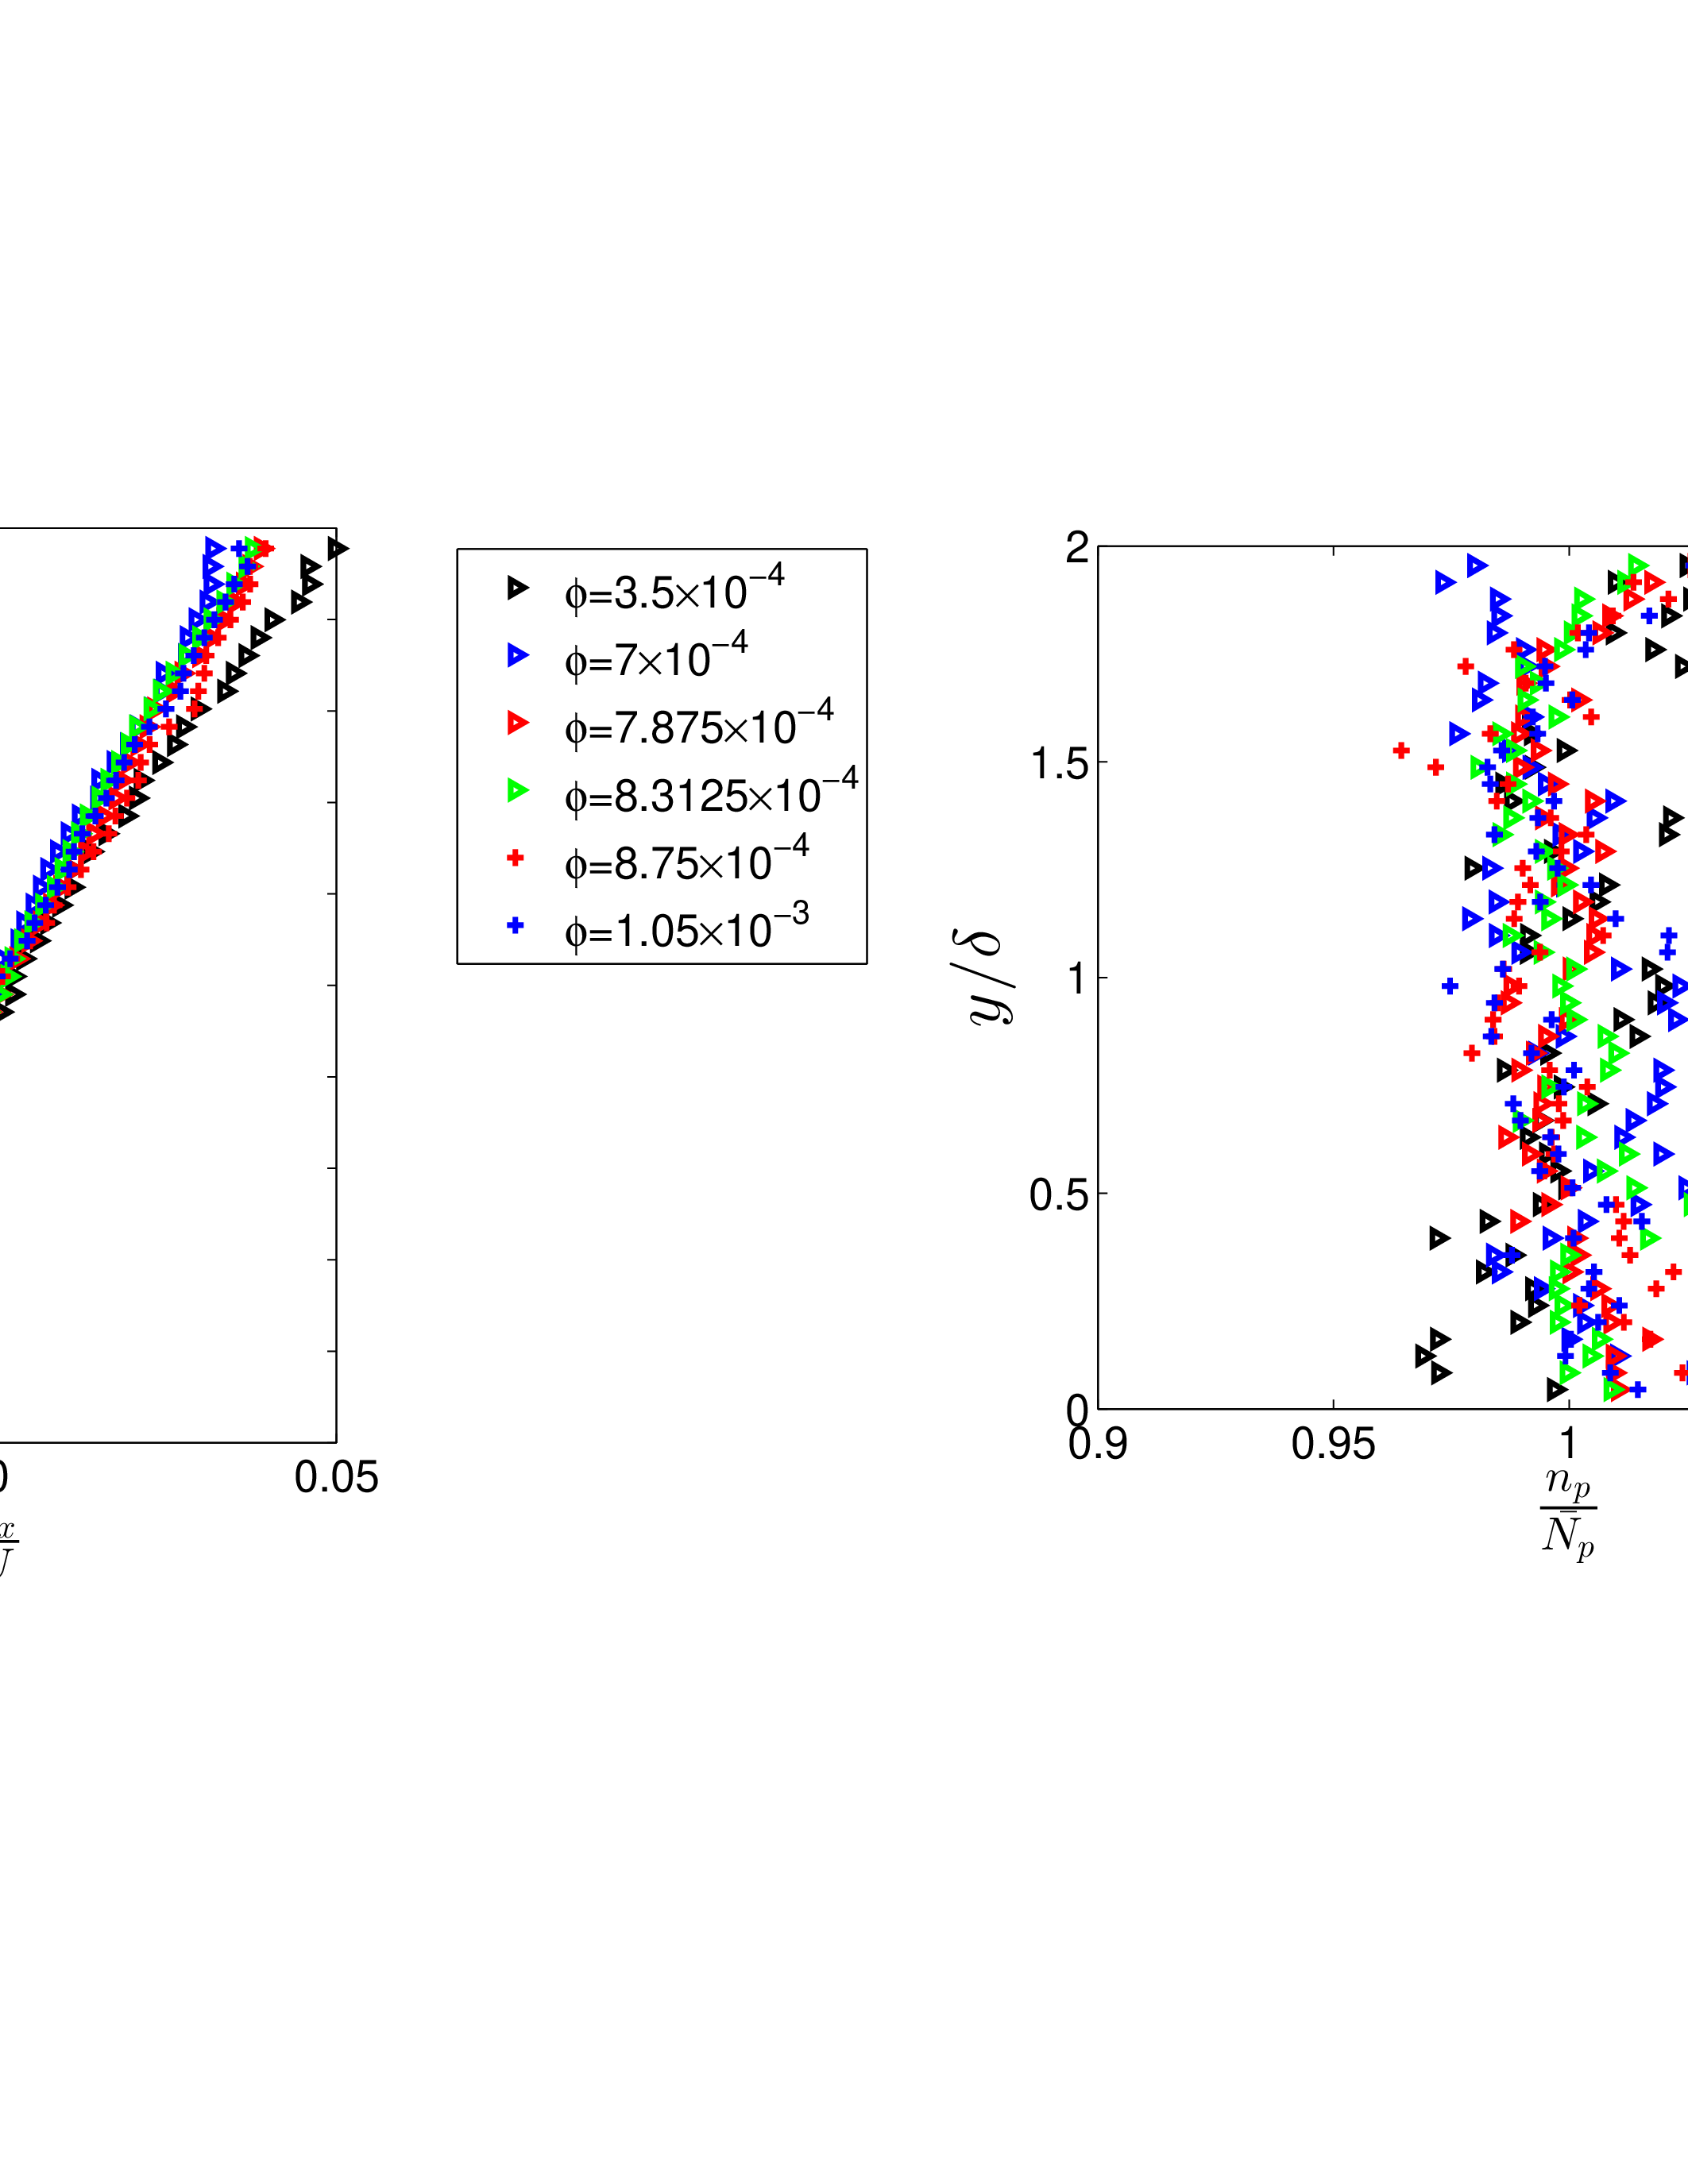}
			\caption{Effect of Particle Volume Fraction on (a) Mean Velocity,(b) Particle Number Concentration and (c) Mean Angular Velocity of the Particle Phase for Inelastic Collisions with $e=0.9$} 
			\label{fig:particle_phase_stat_1_inelastic}
		\end{figure}
This subsection contains the particle phase statistics when the inter-particle and wall-particle collisions are slightly inelastic with $e-0.9$. Mean velocity, particle concentration profiles, and the second moments of the velocities show trends similar to the elastic ideal collisions. It is observed here as well as in \ref{chapt2} section \ref{sec:inelastic} that the cross-stream velocity fluctuations of the particles decrease significantly. Here a slight inelasticity lowers the cross-stream velocity fluctuations by $40-50\%$. Other statistics show little to marginal variation with inelasticity. 		
		\begin{figure}[!h]
			\includegraphics[width=1.0\textwidth,  height=9cm]{app/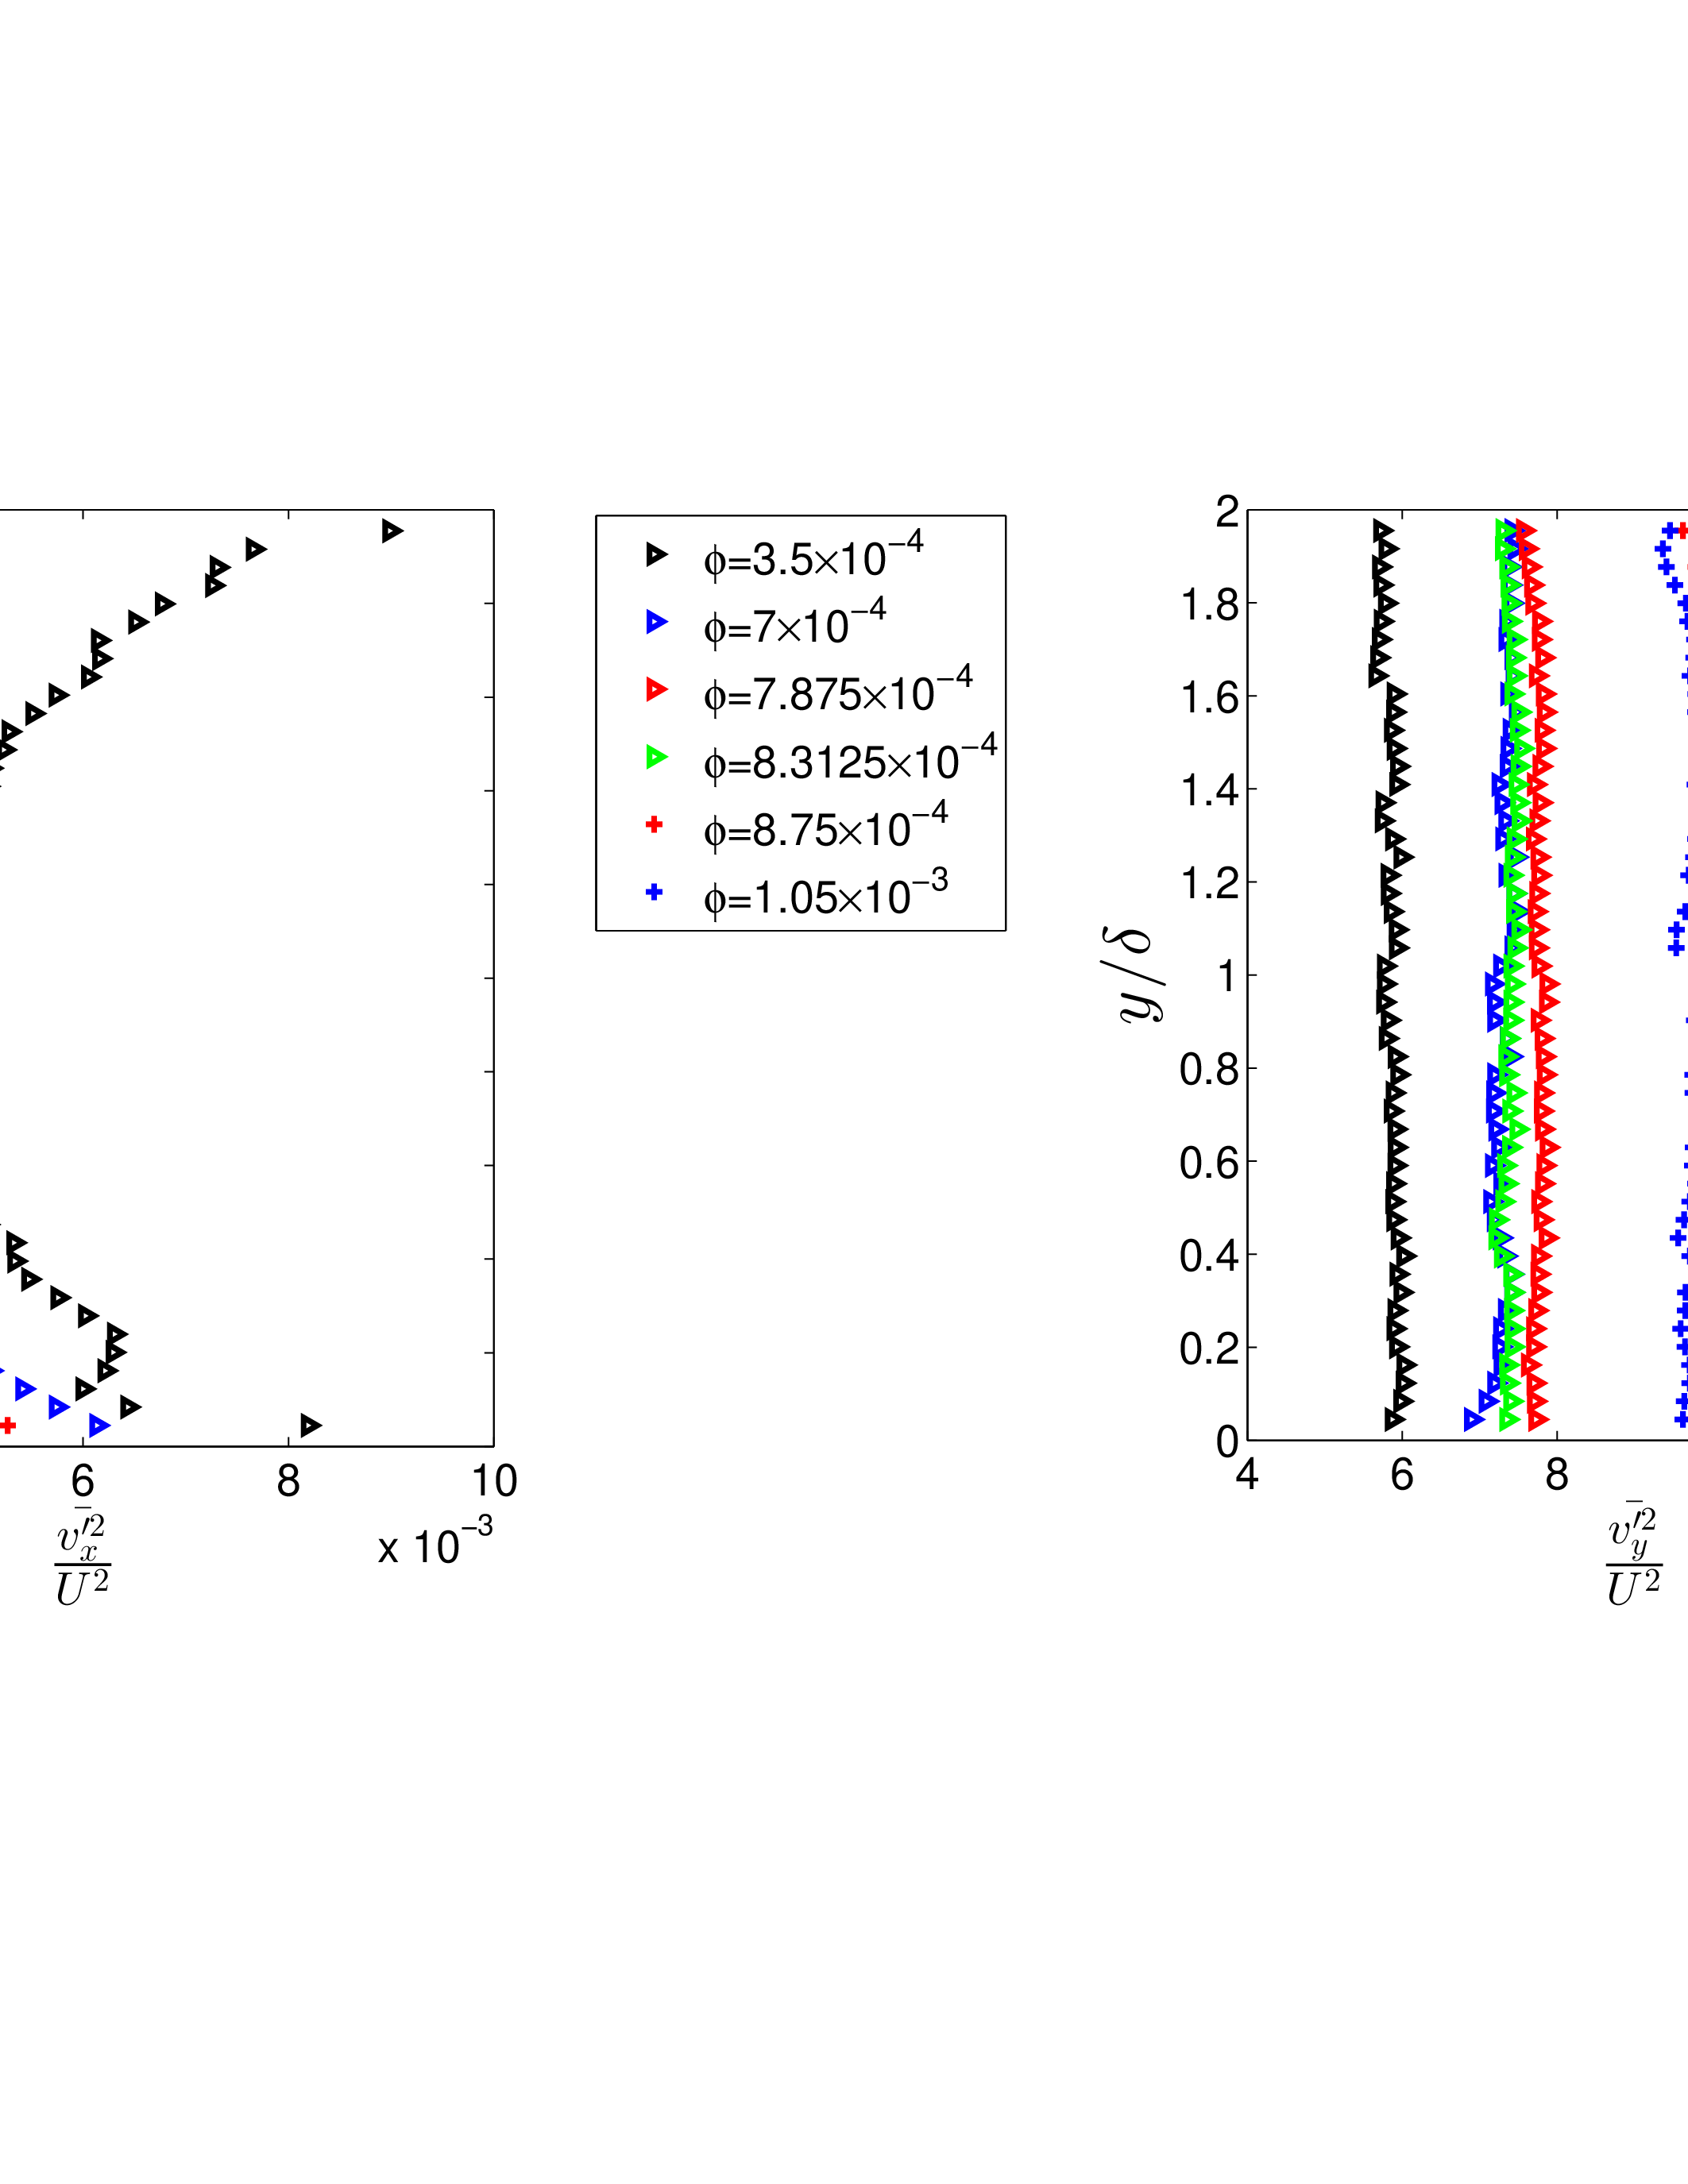}
			\caption{Effect of Particle Volume Fraction on (a) Stream-wise and (b) Cross-stream Mean Square Velocity of the Particle Phase for Inelastic Collisions with $e=0.9$}
			\label{fig:particle_phase_stat_2_inelastic}
		\end{figure} 
		\begin{figure}[!h]
			\includegraphics[width=1.0\textwidth,  height=9cm]{app/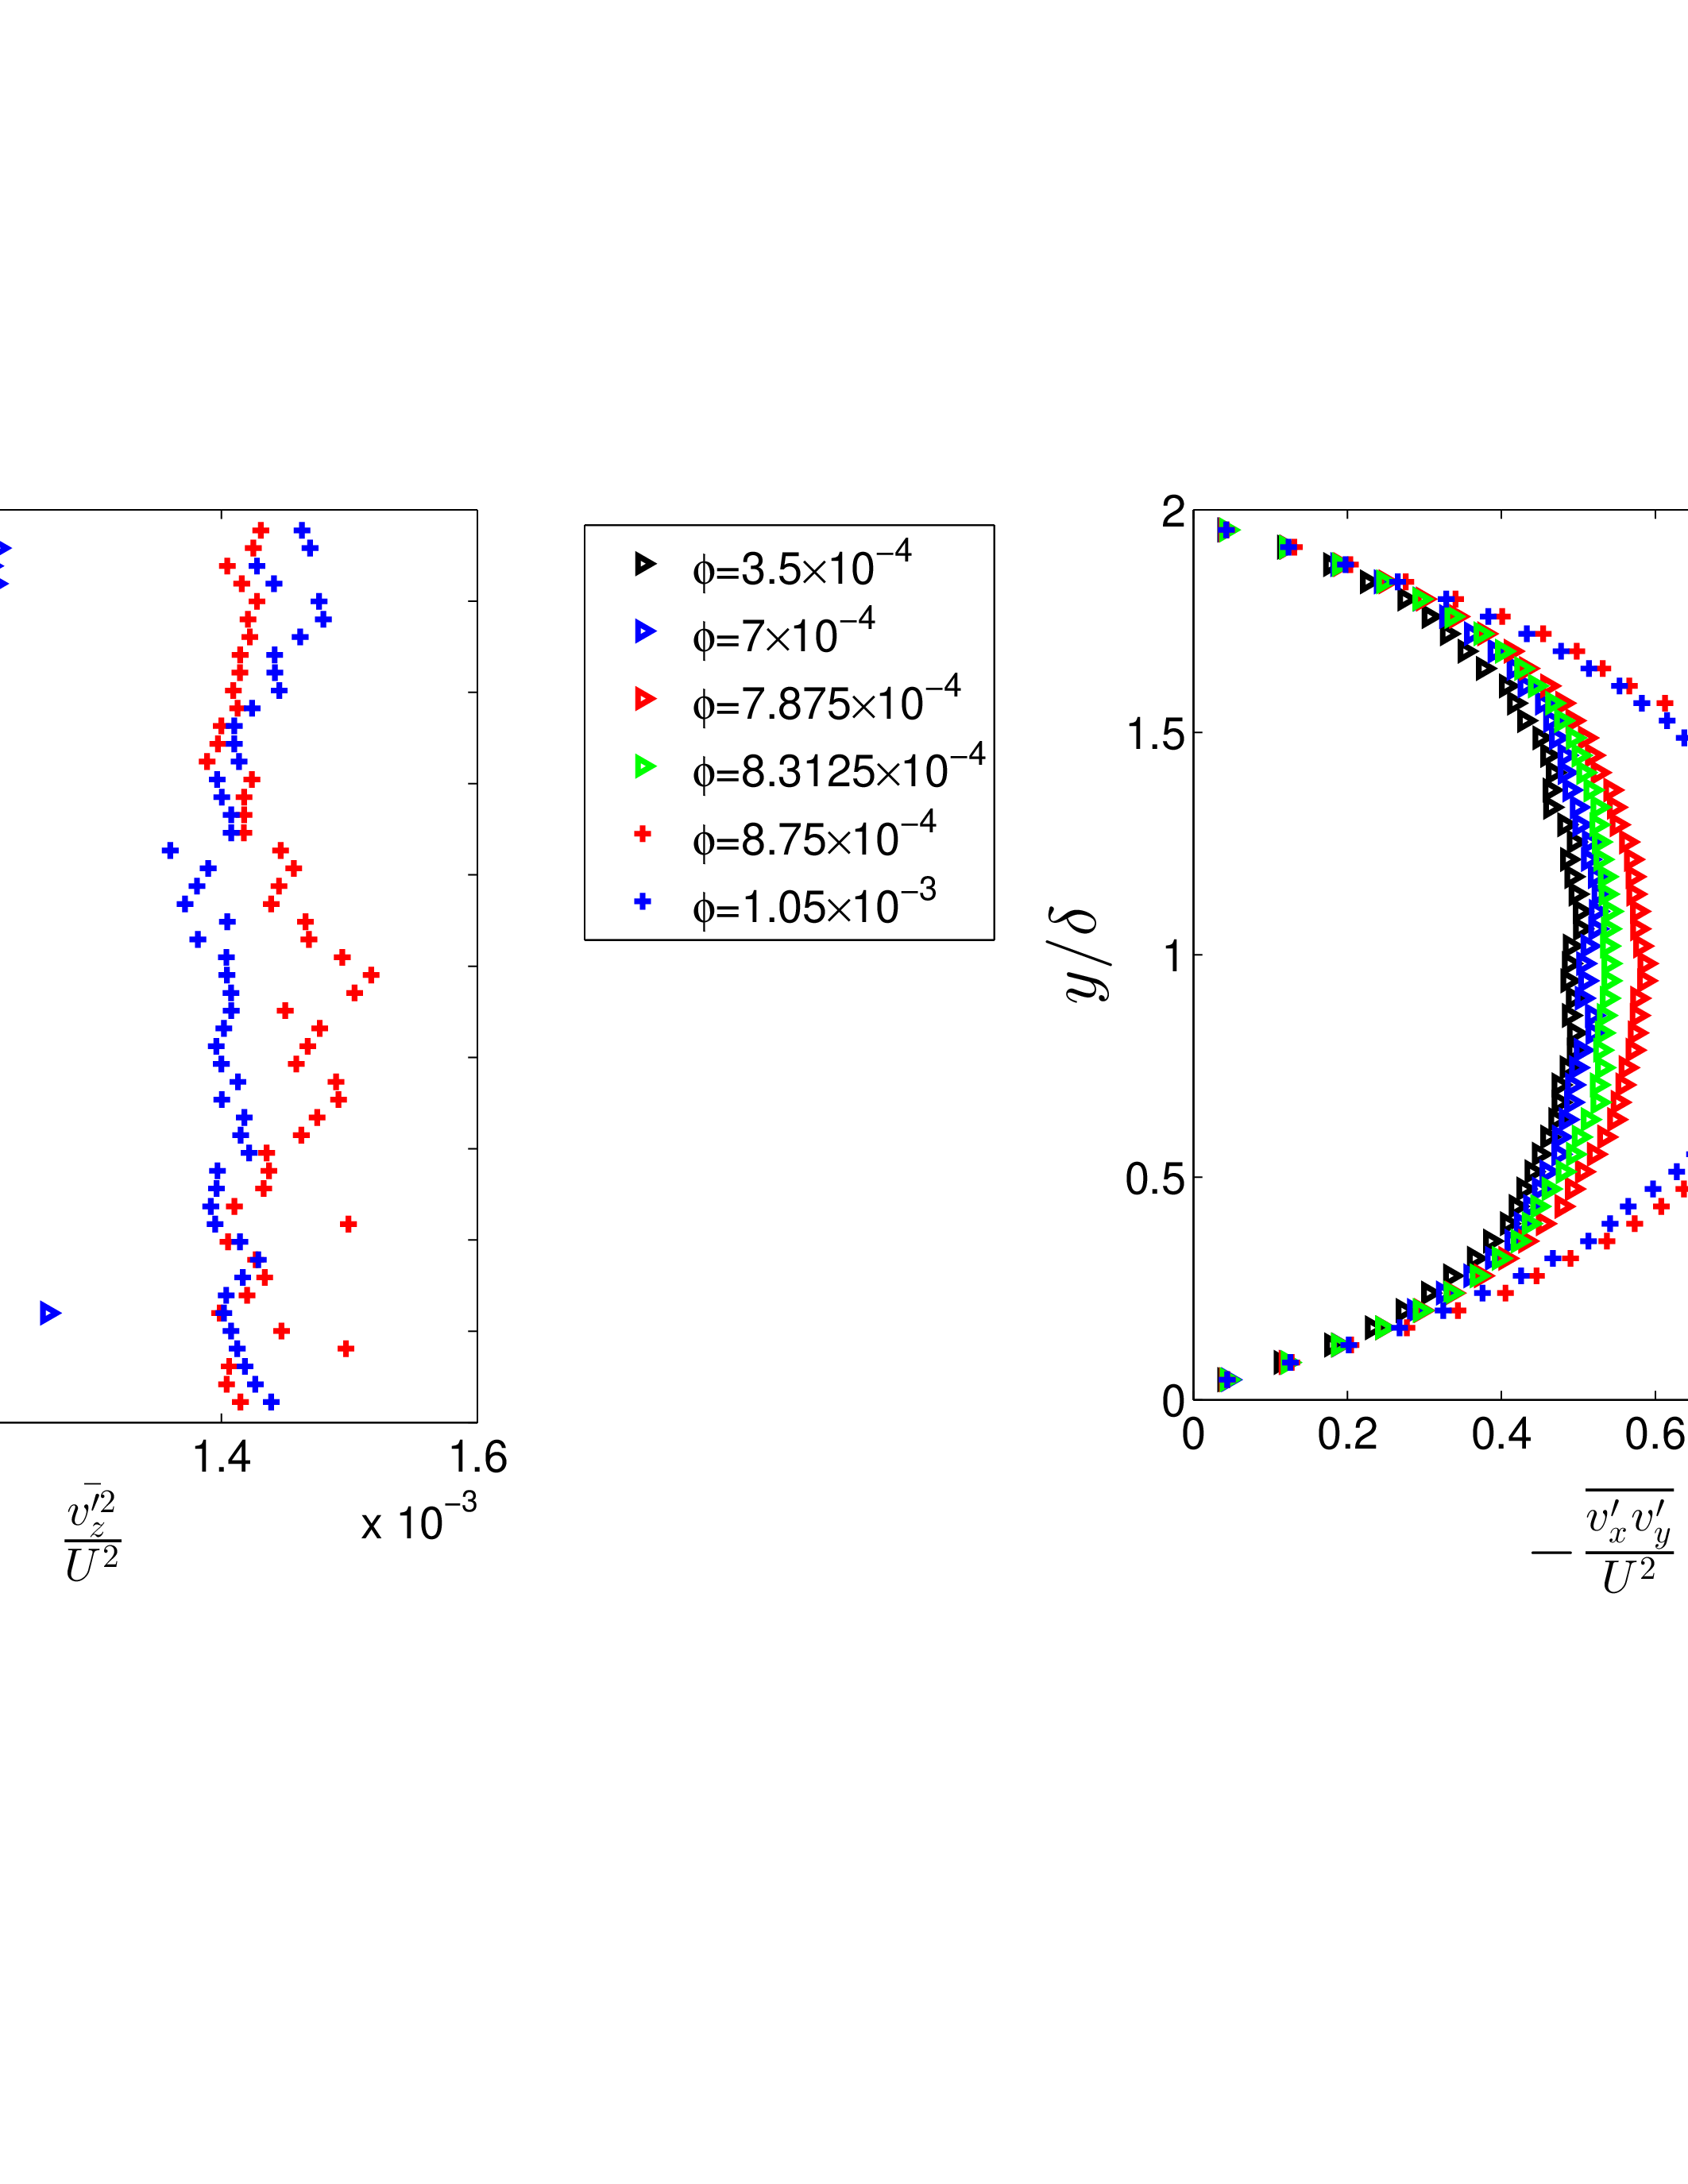}
			\caption{Effect of Particle Volume Fraction on (a) Span-wise Mean Square Velocity, (b) Stream-wise and Cross-stream Velocity Cross-correlation of the Particle Phase for Inelastic Collisions with $e=0.9$} 
			\label{fig:particle_phase_stat_3_inelastic}
		\end{figure}

\clearpage
\subsection{Particle Phase Statistics in Absence of Inter-particle Collisions}
\label{sec:Particle Phase Statistics zero_coll}
The hypothetical study of switching off the inter-particle collisions, as discussed in section \ref{sec:zero_coll}, bring about a few interesting and different qualitative behaviour of particle phase statistics especially after the transition in turbulence. After the transition, unlike any cases discussed before, particle mean velocity do not show any slip at the walls along with a very high mean velocity gradient near the walls (Fig.\ref{fig:particle_phase_stat_1_zero_coll}(a)). The particles tend to accumulate more in the near-wall region for suspension above critical volume fraction, although very little variation of particle concentration is observed before transition (Fig. \ref{fig:particle_phase_stat_1_zero_coll}(b)). Due to the absence of inter-particle collisions the redistribution of particle x momentum to y and z direction gets drastically decreased. Hence we observe span-wise and cross-stream particle mean square velocities and covariance $\overline{v_x'v_y'}$ drastically decrease.  This decrease is about two-orders of magnitude for $\bar{v_y'^2}$ and $\bar{v_z'^2}$ and one-order of magnitude for $\overline{v_x'v_y'}$ with respect to the ideal collisional condition shown in section\label{sec:Particle Phase Statistics}. 
% Decrease of $\bar{v_y'^2}$, $\bar{v_z'^2}$ with respect to $\phi$ is also due to the absence of collision and a direct result of fluid-particle coupling.
The most interesting trend is observed for $\bar{v_x'^2}$. Increase in $\bar{v_x'^2}$ values with a completely different trend, i.e. zero at the walls and maximum at the centre, occur after the transition in turbulence as a result of the  shear induced particle migration. Hence the different trends are found to be independent with small changes in volume fraction as well. \textcolor{blue}{Following analysis suggests that the streamwise fluctuation of the particle phase in the absence of particle-particle collision originates from the wall normal migration of the particles under sheared velocity profile. In this mechanism, the magitude of streamwise velocity fluctuation ($v_x'$) induced, can be written as:
\begin{equation}
    v_x'\approx\sqrt{\overline{v_y'^2}}\tau_v \frac{\partial U}{\partial y}
\end{equation} 
For, $\phi=9.625\times10^{-4}$, at $y=\delta$, $\overline{v_x'^2}=1.468\times10^{-6}$; average mean velocity gradient $\frac{\partial U}{\partial y}\approx1.0$
and $\tau_v=367$ yields 
\begin{math}
v_x'\approx 0.448
\end{math}
or, 
\begin{math}
\overline{v_x'^2}\approx 0.19
\end{math}. 
This is of the same order of magnitude as observed from the Fig. \ref{fig:particle_phase_stat_2_zero_coll}(b) which is around 0.14.}

\begin{figure}[!h]
			\includegraphics[width=1.0\textwidth,  height=9cm]{app/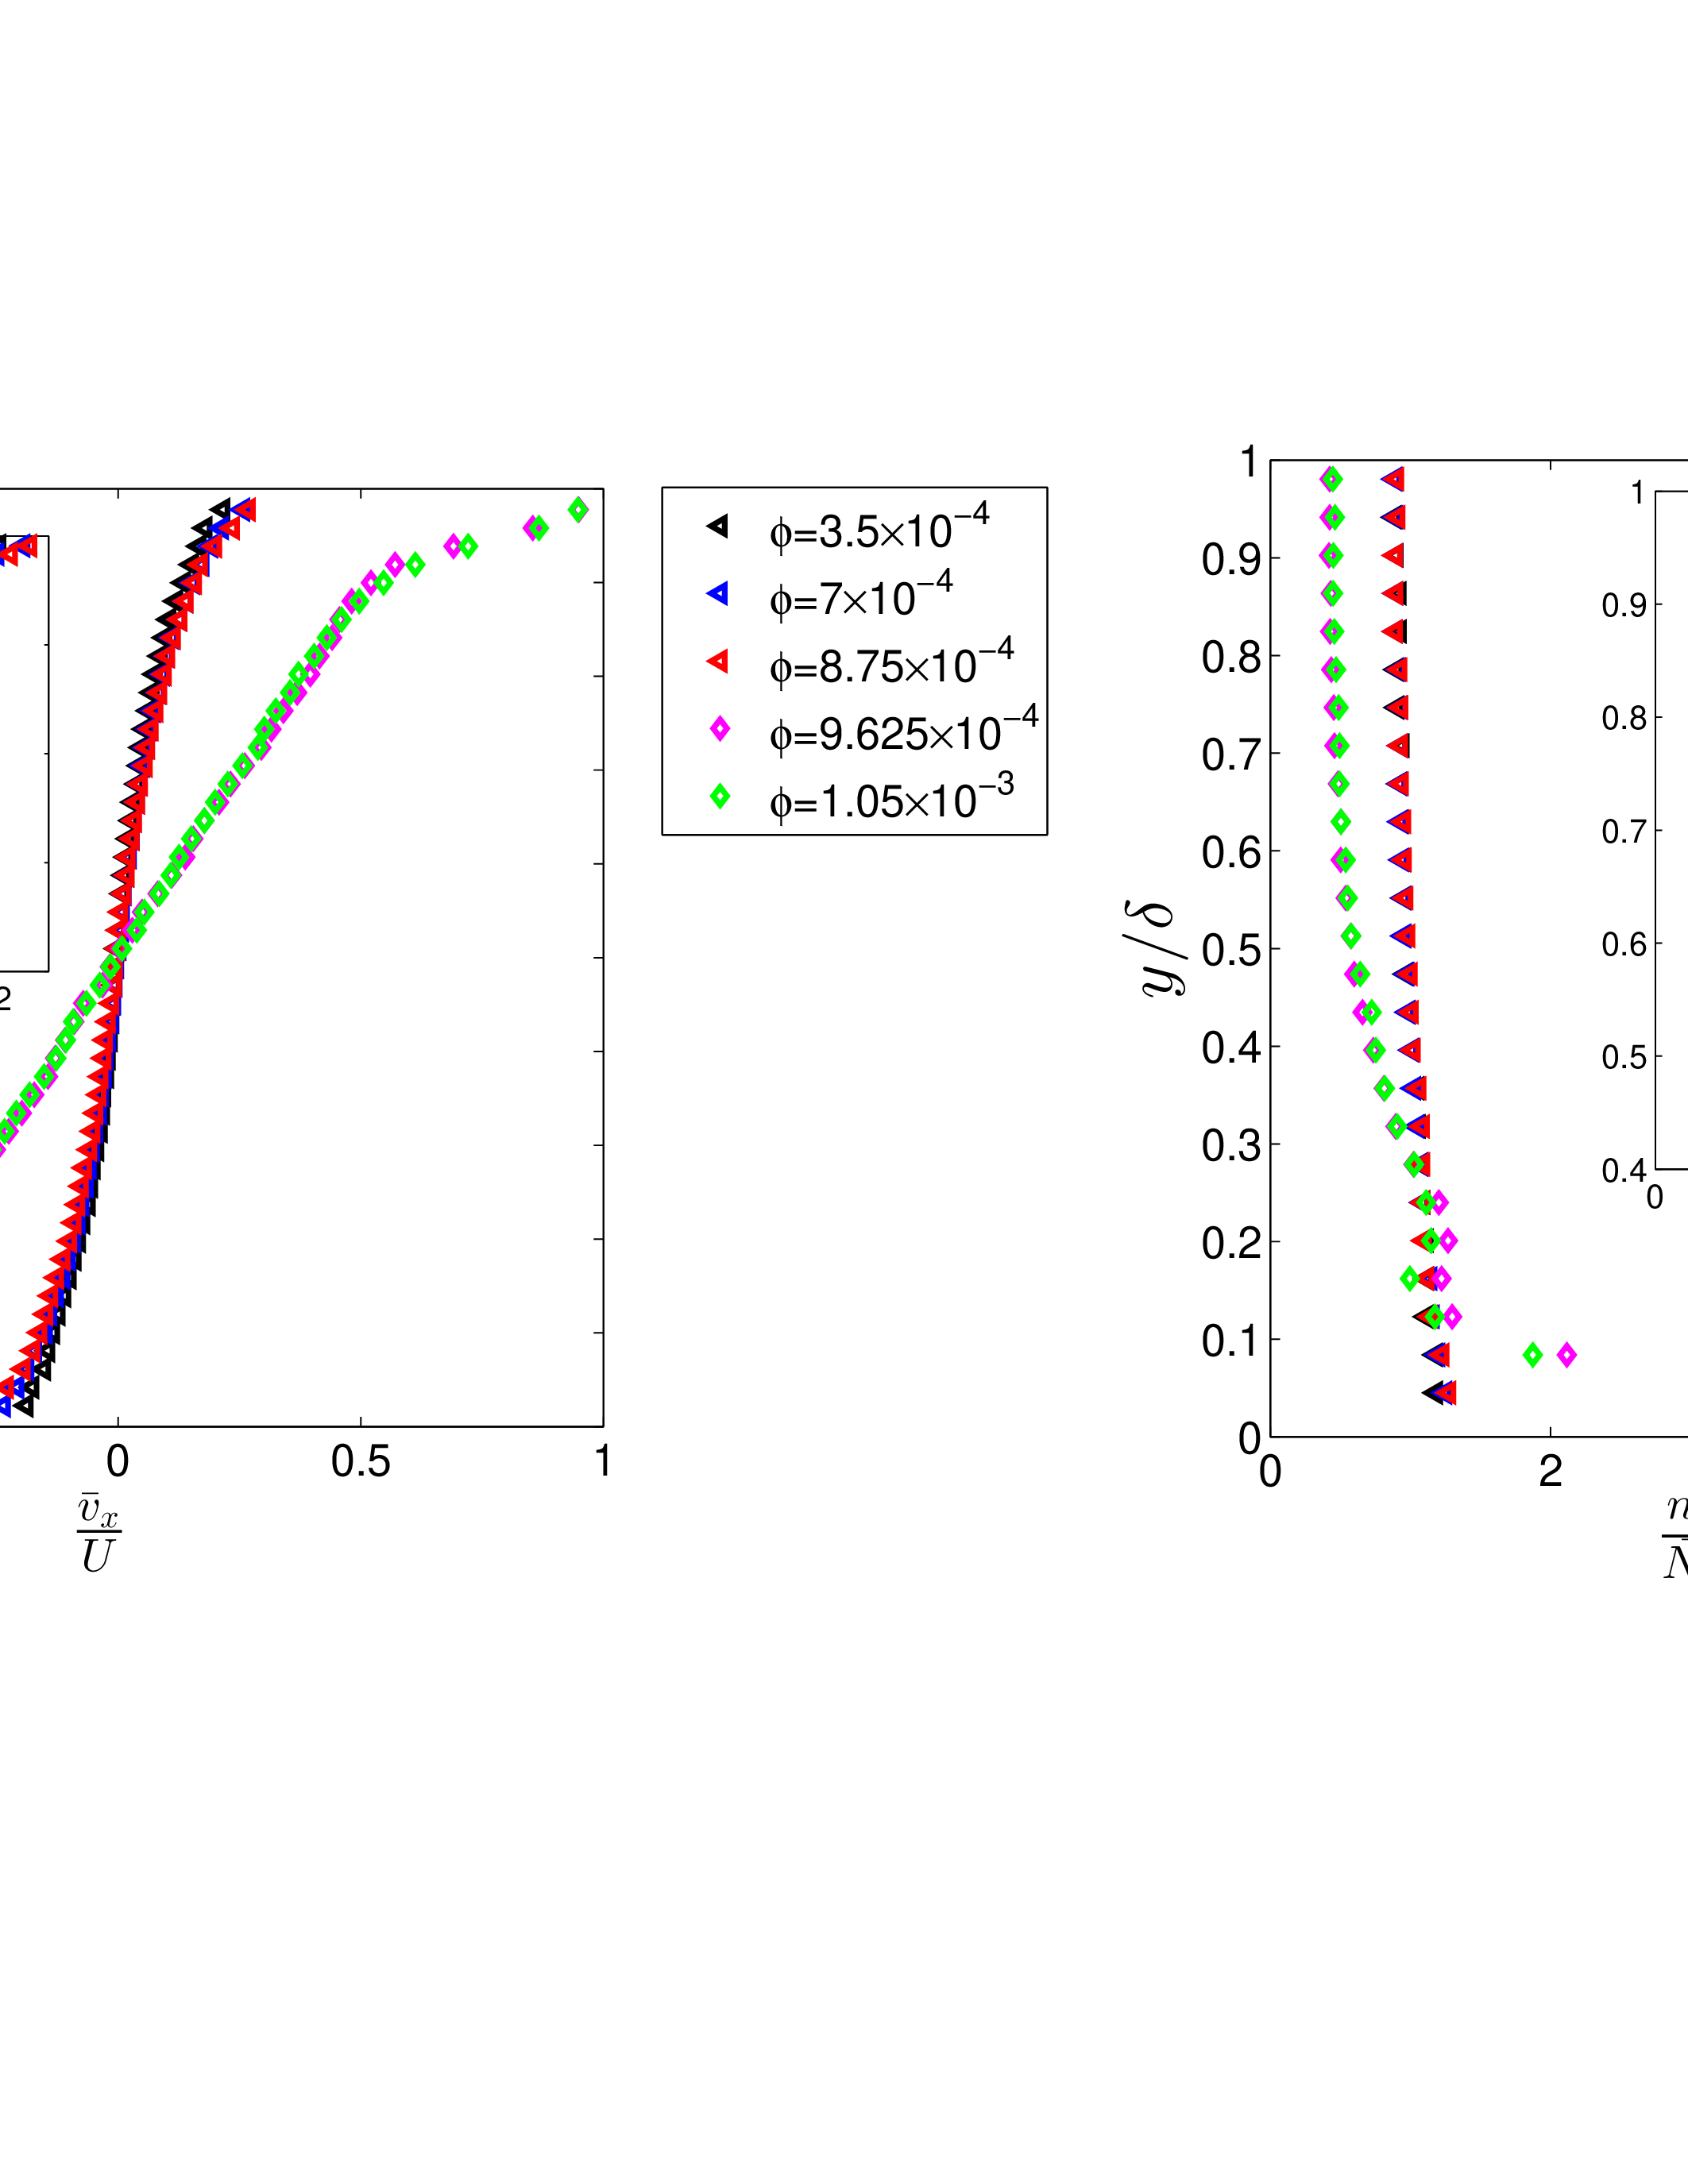}
			\caption{Effect of particle volume fraction on (a) mean velocity,(b) particle number concentration and of the particle phase in absence of inter-particle collisions} 
			\label{fig:particle_phase_stat_1_zero_coll}
		\end{figure}
		
		\begin{figure}[!h]
			\includegraphics[width=1.0\textwidth,  height=9cm]{app/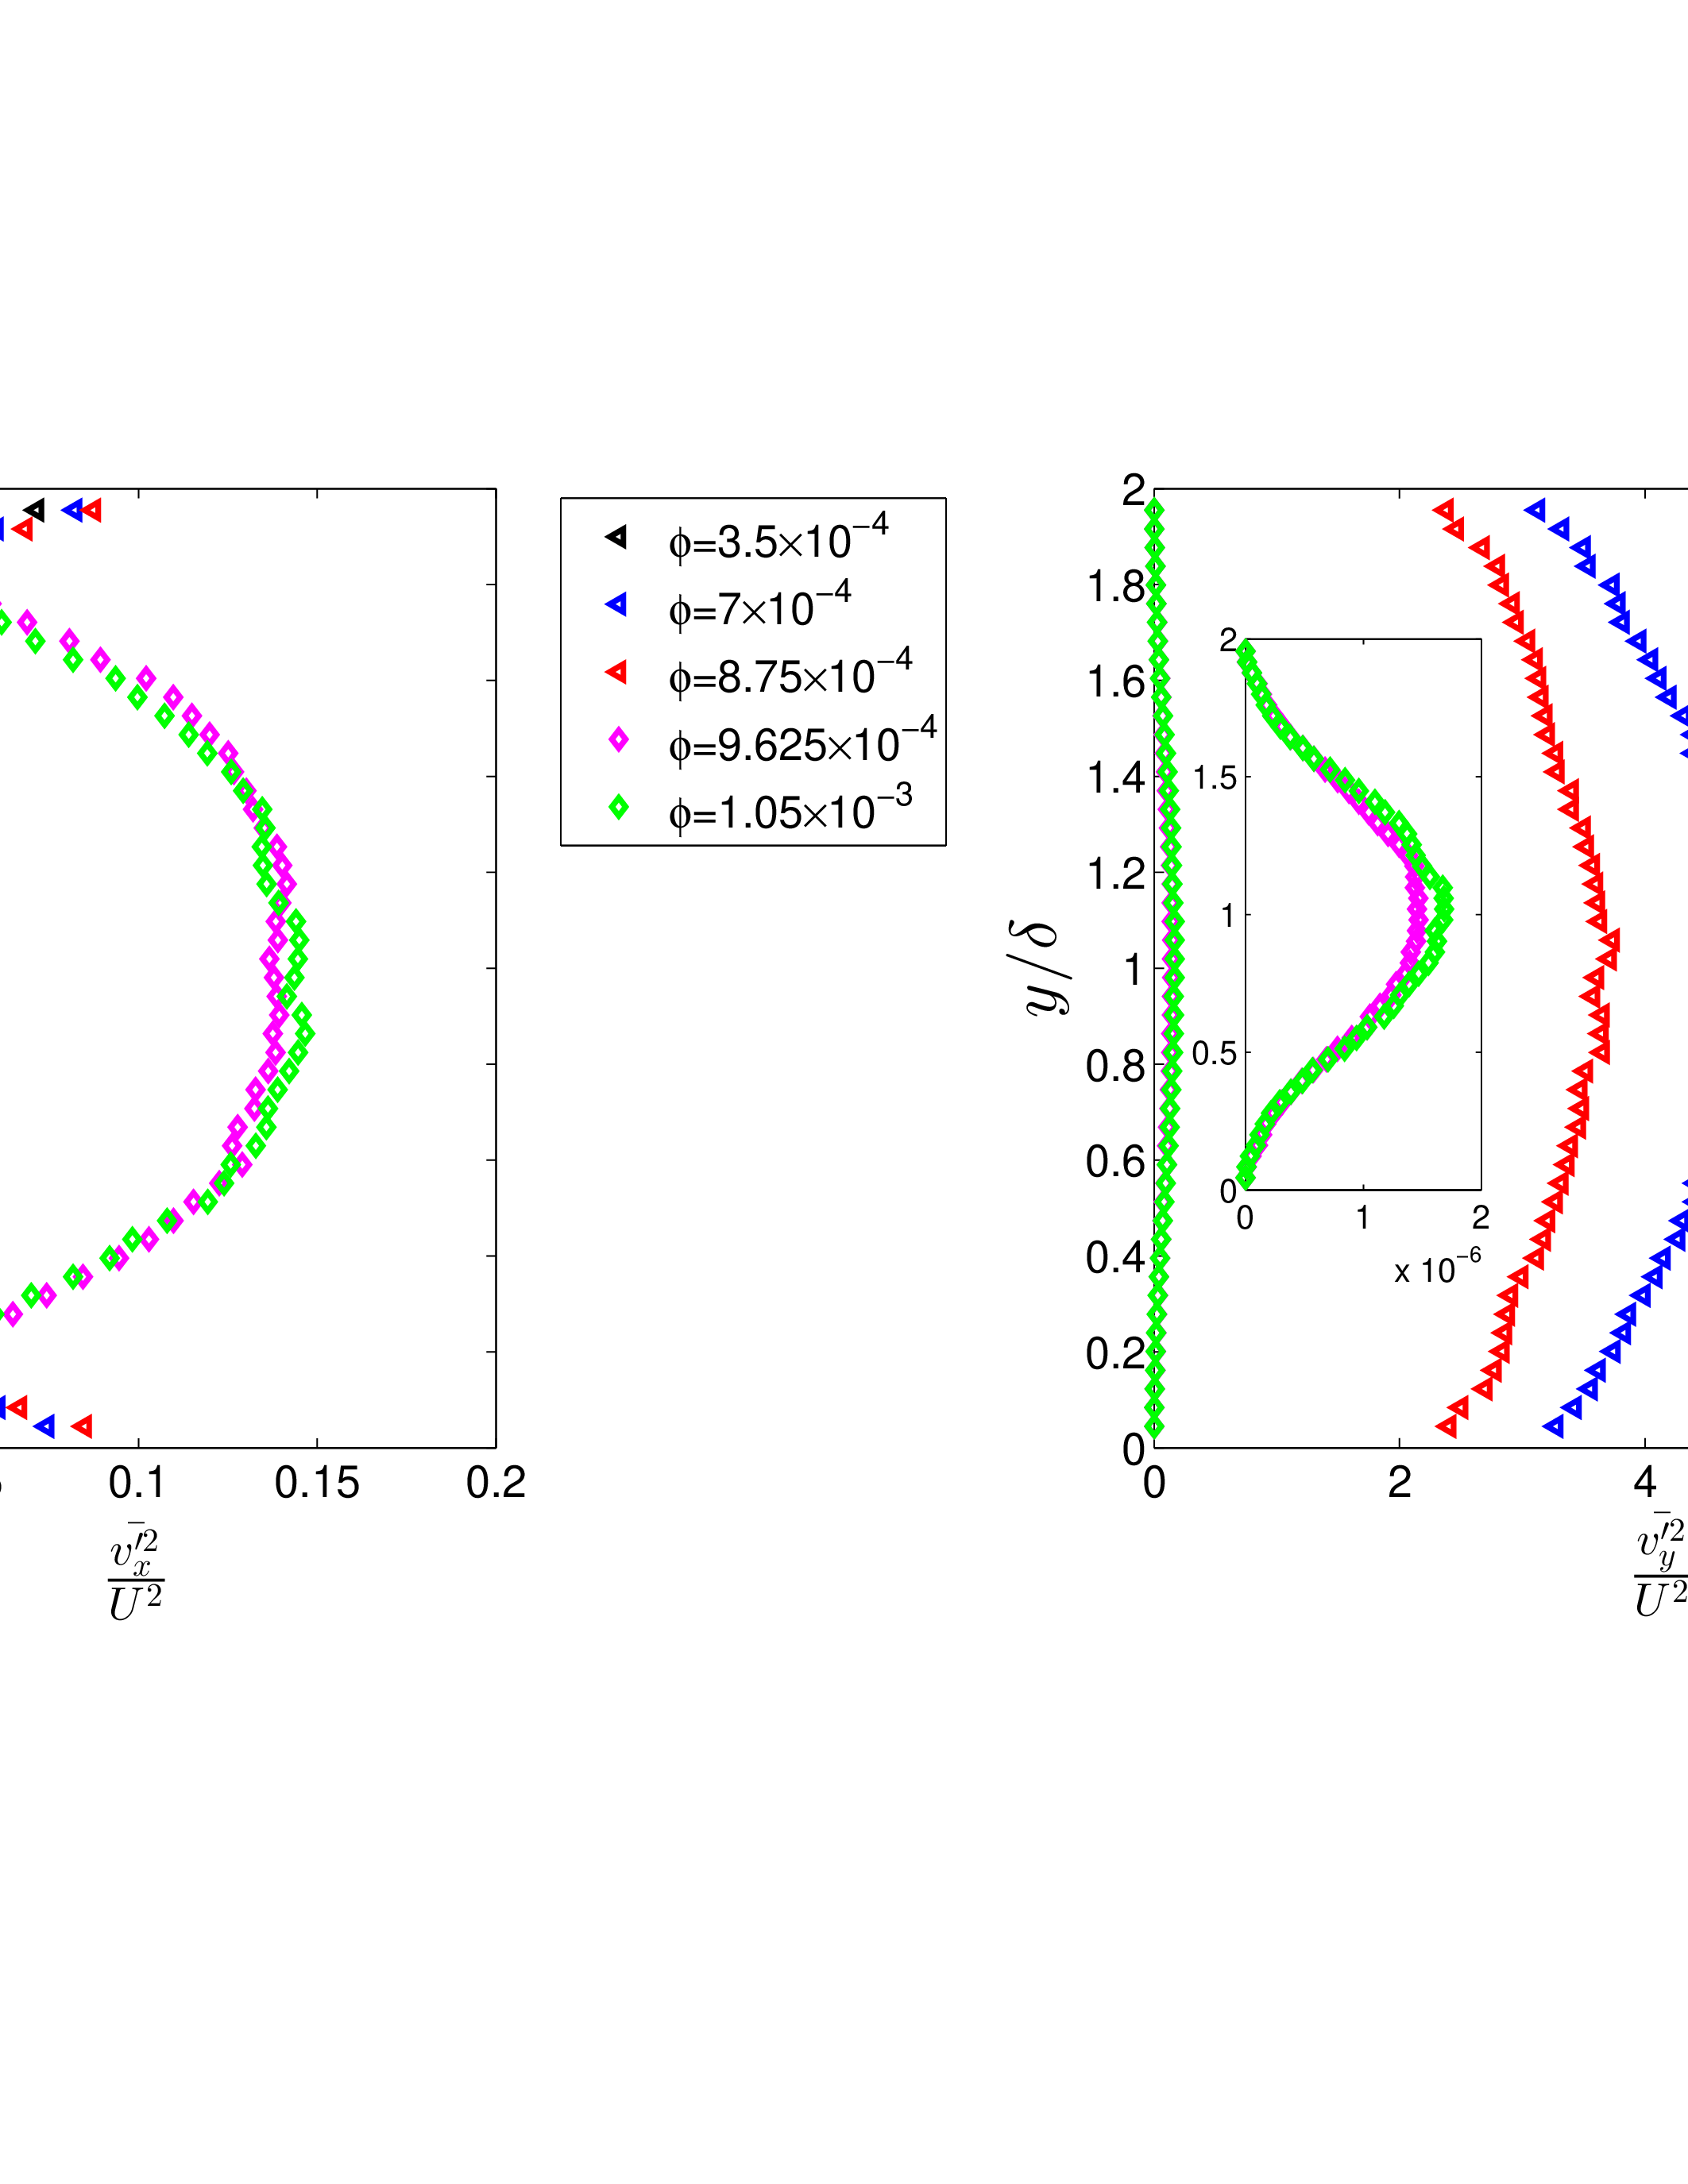}
			\caption{Effect of particle volume fraction on (a) stream-wise and (b) cross-stream mean square velocity of the particle phase in absence of inter-particle collisions}
			\label{fig:particle_phase_stat_2_zero_coll}
		\end{figure} 
		\begin{figure}[!h]
			\includegraphics[width=1.0\textwidth,  height=9cm]{app/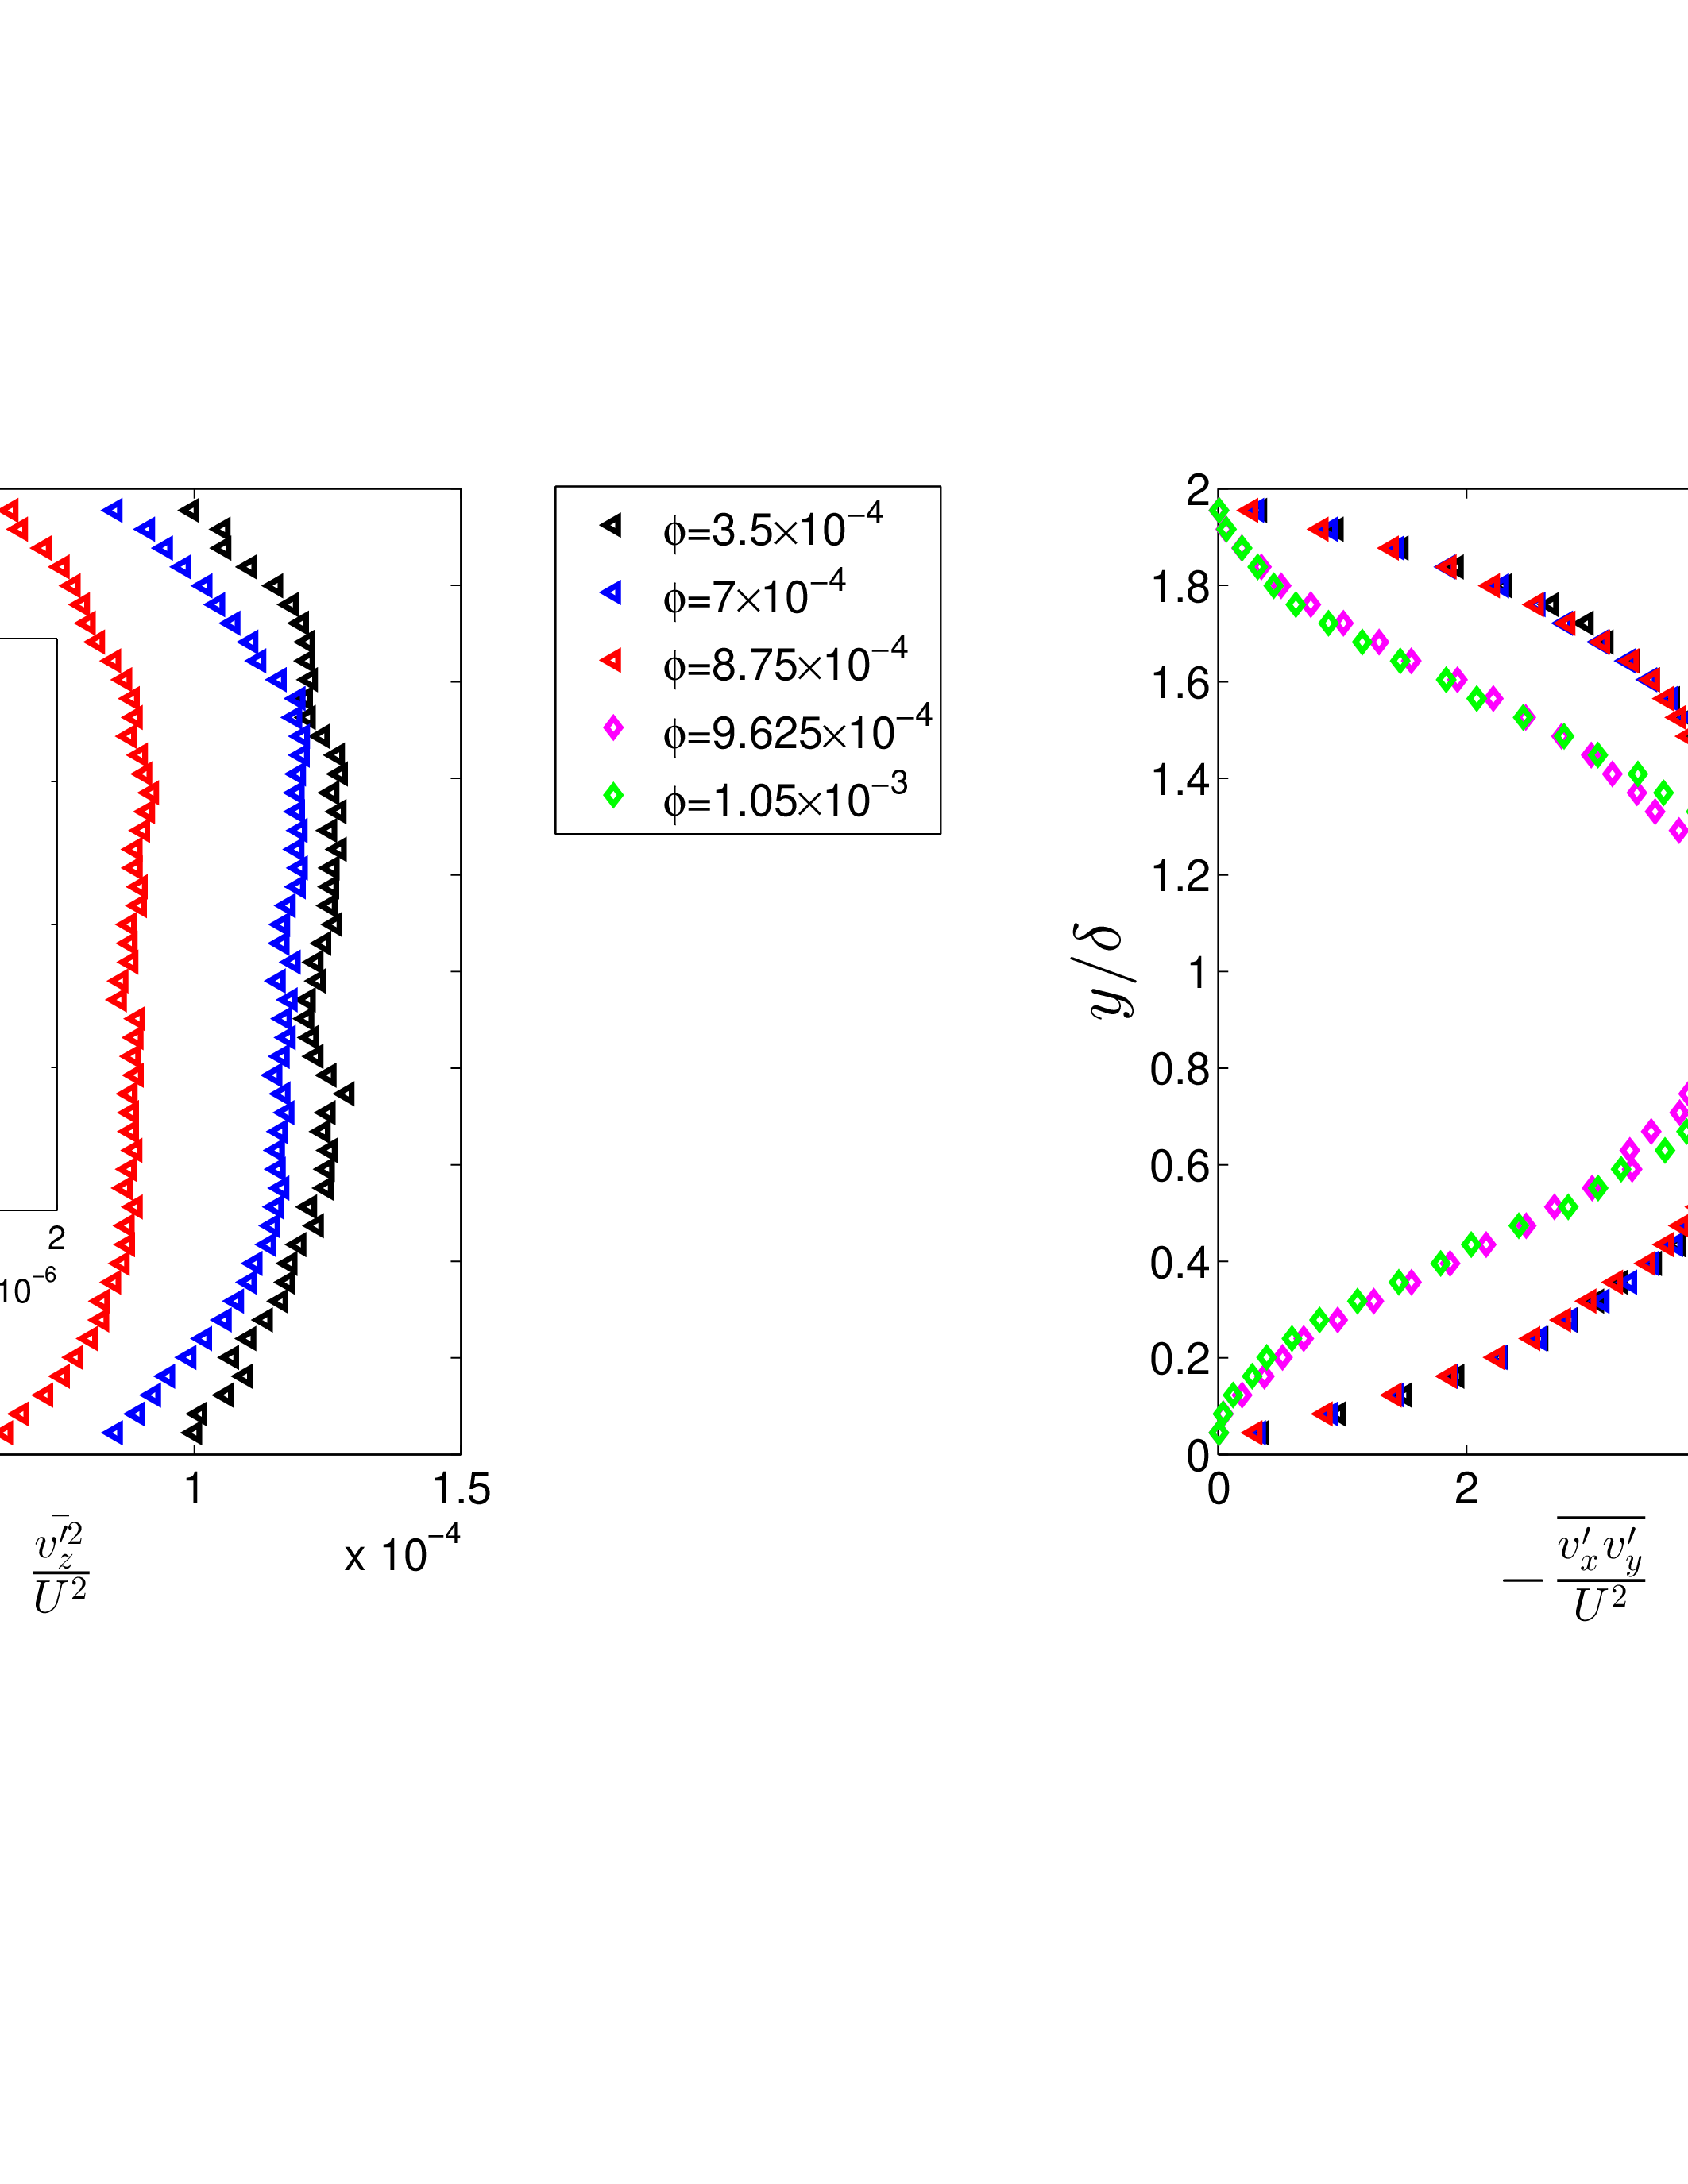}
			\caption{Effect of particle volume fraction on (a) span-wise mean square velocity, (b) particle phase shear stress in the  absence of inter-particle collisions} 
			\label{fig:particle_phase_stat_3_zero_coll}
		\end{figure}
   Thus the the particle-phase statistics along with the fluid phase statistics take a very important role in understanding two-way coupled turbulent suspensions in absence of collisions.
